# Supplementary material for: iFDK: A Scalable Framework for Instant High-resolution Image Reconstruction
Source: arXiv:1909.02724 source file (2019-09-06)
Supplement: Supplementary file 1 [file appendix.tex]

%% Appendix
\newpage
\appendix
\section{APPENDIX}\label{appendix}
%\subsection{Provement}\label{Provement}
In this appendix, we prove that in the specified rotation angle $\beta$, if the $\hat{i}$ and $\hat{j}$ are fixed, the $z$ in Equ~\ref{equ:uv} is a constant value.
As Fig~\ref{fig:CT.geometry} shown, given a point a of coordinate $(\tilde{i}, \tilde{j}, \tilde{k})$ in volume coordinate system, its projection point A of coordinate $(u, v)$ on the FPD can be computed via projection equation:
\begin{equation}
	\label{equ:uv}
    \left\{
    \begin{alignedat}{4}
        [x,y,z]^T &= P_\beta\cdot[\tilde{i}, \tilde{j}, \tilde{k}, 1]^T\\
        [u,v]^T &= [x,y]^T\cdot 1/z
    \end{alignedat}
    \right.
\end{equation}
where x,y,z are temporary variables. $P_i$ is the $3{\times}4$ projection matrix on the condition that gantry rotation angle is $\beta$. Hence, the $P_i$ can be derived as
\begin{equation}
    \left\{
    \begin{alignedat}{4}
                    \beta &= i{\cdot}\theta\\    
        \hat{P}_i &= M_1{\cdot}M_{rot}{\cdot}M_0\\
                    P_i &= \hat{P}_i[0:3]\\
    \end{alignedat}
    \right.
\end{equation}
where the shapes of $\hat{P}_i$ and $P_i$ are $4\times4$ and $4\times3$, respectively. $M_0$, $M_{rot}$, and $M_1$ are listed as following
\begin{equation*}
\setlength{\arraycolsep}{3pt}
\scriptsize
M_0=
\begin{pmatrix}
		D_x&      0&       0&      0\\
		0&       D_y&      0&      0\\
		0&       0&       D_z&     0\\
		0&       0&       0&       1\\
\end{pmatrix}
\cdot
\begin{pmatrix}
		1&  0&  0& -\frac{N_x-1}{2.0}\\
		0& -1&  0& \frac{N_y-1}{2.0}\\
		0&  0& -1& \frac{N_z-1}{2.0}\\
		0&  0&  0&            1 \\
\end{pmatrix}
\end{equation*}

\begin{equation*}
\setlength{\arraycolsep}{3pt}
\scriptsize
M_{rot}=
\begin{pmatrix}
		1&       0&       0&       0\\
		0&       0&      -1&       0\\
		0&       1&       0&       d\\
		0&       0&       0&       1\\
\end{pmatrix}
\cdot
\begin{pmatrix}
		cos(\beta)&  -sin(\beta)&       0&       0\\
		sin(\beta)&   cos(\beta)&       0&       0\\
		0&                     0&       1&      0\\
		0&                     0&       0&       1
\end{pmatrix}
\end{equation*}

\begin{equation*}
\setlength{\arraycolsep}{3pt}
\scriptsize
M_{1}=
\begin{pmatrix}
		\frac{1}{D_u}&         0&             0&       0\\
		0&         \frac{1}{D_v}&             0&       0\\
		0&                     0&             1&       0\\
		0&                     0&             0&       1
\end{pmatrix}
\cdot
\begin{pmatrix}
		D&  0&  \frac{(N_u-1){\cdot}D_u}{2}&  0\\
		0&  D&  \frac{(N_v-1){\cdot}D_v}{2}&  0\\
		0&  0&                          1&  0\\
		0&  0&                          0&  1
\end{pmatrix}
\end{equation*}
$M_0$ means transforming the coordinate system from volume to gantry, $M_{rot}$ denotes gantry rotate along $Z$ axis of angle $\beta$ plus transpose distance $d$, $M1$ indicates projecting point to FPD plane. Note that all of the variable are listed in Table~\ref{tbl:cbct-param}. $\cdot$ indicates matrix multiplication.

by expanding Equ.~\ref{equ:uv}, the value $z$ is
\begin{equation}
\label{equ:z}
z = d+sin(\beta)(\tilde{i}-\frac{N_x-1}{2})D_x-cos(\beta){\cdot}(\tilde{j}-\frac{N_y-1}{2})D_y
\end{equation}
clearly, $z$ is independent to value $\hat{k}$, and equal to $d+y_{ab}$, where $y_{ab}$ is the Y coordinate of line $\overline{ab}$, which is parallel to Z-axis.
